# Supplementary material for: Simple subvector inference on sharp identified set in affine models
Source: arXiv:1904.00111 source file (2024-07-24)
Supplement: Supplementary file 1 [file Outline.tex]

\subsection{Outline}

 \subsubsection{Plan of the Lemmas}

 Lemma \ref{lem:LICQ} proves that Assumption \ref{assu:NoOveridentification}
 is equivalent to Assumption \ref{assu:LICQ}. Linear Independence
 constraint Qualification is a necessary and sufficient condition for
 uniqueness of Lagrange multipliers in programs (\ref{prog:minP}),(\ref{prog:regProg}),
 and (\ref{eq:DualProgram0}). 

 Lemma \ref{lem:UniqueMin} provides a representation of the minima
 to (\ref{prog:minP}) and (\ref{prog:regProg}) as a solution to a
 KKT system. The KKT representation is used by the numerical software
 that finds the minima as a solution to the conditions. Lemma \ref{lem:UniqueMin}
 also has a bound on the norm of the Lagrange multipliers in terms
 of singular values of the active constraints.

 Lemma \ref{lem:compactPbar} shows that the closure of $\mathcal{P}$
 is compact and satisfies the conditions 1-4 of Definition \ref{def:-DistributionClass}.
 This Lemma is necessary to establish continuity of the solutions in
 both in $\mu$ and $\measTrue\in\mathcal{P}$ in Lemma \ref{lem:continuityInMuP}.
 These continuity properties are crucial for Lemma \ref{lem:DeltaMethod}
 and \ref{lem:FirstCoordinate}. 

 Lemma \ref{lem:UniformLagrangeBound} shows that the Lagrange multipliers
 have a uniformly bounded norm for $\measTrue\in\mathcal{\bar{P}}$.
 The bound only depends on the maximal norm of $\theta$ and $\eta$
 from Definition \ref{def:-DistributionClass}. This bound is used
 Lemmas \ref{lem:continuityInMuP} and \ref{lem:DeltaMethod}.

 In Lemma \ref{lem:continuityInMuP} I show that the solution to the
 KKT system can be represented as a solution to a least squares problem.
 It allows me to use the Maximum theorem to establish continuity of
 Lagrange multipliers for any $\mu\geq0$ and $\measTrue\in\mathcal{P}$
 and the hemicontinuity of the argmin. 

 Lemma \ref{lem:compactP} uses Lemma \ref{lem:continuityInMuP} to
 show that any point in $\mathcal{P}$ satisfies the condition 5 of
 Definition \ref{def:-DistributionClass}. This result is important
 for Lemma \ref{lem:DeltaMethod} to avoid devision by a zero variance. 

 Lemma \ref{lem:directionalDerivative} establishes that the change
 in the solution to the regularized program is linear in size of the
 perturbation. This result gives directional derivatives for any change
 in the coefficients of the constraints and $\mu$. The perturbation
 in $\mu$ corresponding to $\alpha_{\delta}\neq0$ is used in Lemma
 \ref{lem:constantTheta}. The perturbation with $\delta\left(\theta\right)\neq0$
 is used in the Delta\textendash method to derive the asymptotic Gaussian
 distribution of the estimator.

 Lemma \ref{lem:2ndorderPert} provides explicit bounds on the error
 due to linear approximation. This result is important to prove asymptotic
 Gaussianity of the bound estimator and consistency of the variance
 estimator in \ref{lem:DeltaMethod}.

 Lemma \ref{lem:constantTheta} is crucial to show that the bias correction
 is exact for any fixed DGP.

 Lemma \ref{lem:FirstCoordinate} shows that the bias $\eOneVec[\prime]\funLArg-\funLValO$
 is zero for $\mu<\mu_{1}$. This result is important in Theorem 2,
 since limit of $\funLArg[\mu_{n}][\measSec]$ depends on the sequence
 $\measSec$. 

 The prerequisite for the Delta method, Uniform LLN and FCLT, are proven
 in Lemma \ref{lem:FCLTandULLN}. They follow immediately from the
 uniform bound on the moments and linearity in $\theta$ on a compact
 set $\Theta$. 

 Lemma \ref{lem:DeltaMethod} puts uses differentiability of the value
 function and the uniform bound on the error to derive uniform convergence
 to a Gaussian distribution. 

 Proof of Theorem 1 uses Lemmas \ref{lem:constantTheta}and \ref{lem:DeltaMethod}.
 Theorem 2 uses Lemmas \ref{lem:FirstCoordinate} and \ref{lem:DeltaMethod}.
