# Supplementary material for: Simple subvector inference on sharp identified set in affine models
Source: arXiv:1904.00111 source file (2024-07-24)
Supplement: Supplementary file 2 [file Figures.tex]

% \begin{figure}[H]
% \begin{centering}
% \begin{tabular}{ccc}
% \includegraphics[scale=0.25]{Figures/regular.pdf} & \includegraphics[scale=0.25]{Figures/nearToFlat.pdf} & \includegraphics[scale=0.25]{Figures/Flat.pdf}\tabularnewline
% \end{tabular}
% \par\end{centering}
% \caption{\label{fig:Identified-sets-DGP13}The identified sets for DGP 1-3 in the MC experiment}
% \end{figure}
