# Supplementary material for: Simple subvector inference on sharp identified set in affine models
Source: arXiv:1904.00111 source file (2024-07-24)
Supplement: Supplementary file 3 [file additional_slackness.tex]

\newpage
\section{Relaxing LICQ}

Propsal

Step 1. Estimate a point in the argmax and minimal slack 

\begin{align}
(\hat{\theta}^0_n,\hat{s}^0_n) &=\argmin_{ {\theta}\in\R^{d} } \eOne {\theta} +\mn\ltwo{\theta}^2 + n\ltwo{s}^2 \\
\text{s.t. } & \begin{cases}
\sMean\moment{w_i}{\theta} - s_j =0, & j\in\setEq,\\
\sMean\moment{w_i}{\theta} - s_j \leq0, & j\in\setIneq
\end{cases} 
\end{align}

Step 2.

\begin{align}
\hat{v}_n &=\min_{ {\theta}\in\R^{d} } \eOne {\theta} +\mn\ltwo{\theta-\hat{\theta}^0_n}^2 + n(\ltwo{s}^2-\ltwo{\hat{s}_n^0}^2) \\
\text{s.t. } & \begin{cases}
\sMean\moment{w_i}{\theta} - s_j =0, & j\in\setEq,\\
\sMean\moment{w_i}{\theta} - s_j \leq0, & j\in\setIneq
\end{cases} 
\end{align}

Conjecture 1. 
\begin{equation}
   \sqrt{n} (\hat{\theta}^0_n,\hat{s}^0_n)-(\theta^0,s^0)\to N
\end{equation}{}

\begin{proof}

\begin{align}
(\hat{\theta}^0_n,\hat{s}^0_n) &=\argmin_{ {\theta}\in\R^{d} } \eOne {\theta} +\mn\ltwo{\theta}^2 + n\ltwo{s}^2 \\
\text{s.t. } & \begin{cases}
\sMean\moment{w_i}{\theta} - s_j =0, & j\in\setEq,\\
\sMean\moment{w_i}{\theta} - s_j \leq0, & j\in\setIneq
\end{cases} 
\end{align}

\end{proof}
