# Supplementary material for: Simple subvector inference on sharp identified set in affine models
Source: arXiv:1904.00111 source file (2024-07-24)
Supplement: Supplementary file 4 [file tables.tex]

\begin{center}
\begin{table}[H]
\begin{centering}
\caption{\label{tab:DGP-1-4-summary}MC results for DGP 1-4 .}
\begin{tabular}{|c|c|cc|cc|cc|cc|}
\hline 
 & \multicolumn{1}{c}{} & \multicolumn{2}{c}{$n=100$} & \multicolumn{2}{c}{$n=1000$} & \multicolumn{2}{c}{$n=10000$} & \multicolumn{2}{c|}{$n=100000$}\tabularnewline
\hline 
DGP & $1-\alpha$ & $\mbox{CI}_{\alpha,n}$ & $\widetilde{\mbox{CI}}_{\alpha,n}$ & $\mbox{CI}_{\alpha,n}$ & $\widetilde{\mbox{CI}}_{\alpha,n}$ & $\mbox{CI}_{\alpha,n}$ & $\widetilde{\mbox{CI}}_{\alpha,n}$ & $\mbox{CI}_{\alpha,n}$ & $\widetilde{\mbox{CI}}_{\alpha,n}$\tabularnewline
\hline 
\multirow{4}{*}{1} & 0.90 & 0.8960 & 0.9890 & 0.8995 & 0.9920 & 0.8925 & 0.9925 & 0.9075 & 0.9945\tabularnewline
 & 0.95 & 0.9460 & 0.9955 & 0.9460 & 0.9965 & 0.9445 & 0.9965 & 0.9530 & 0.9970\tabularnewline
 & 0.975 & 0.9705 & 0.9980 & 0.9740 & 0.9980 & 0.9735 & 0.9990 & 0.9745 & 0.9995\tabularnewline
\cline{2-10} 
 & Avg. Ex. Len. & 0.0583 & 0.0888 & 0.0186 & 0.0292 & 0.0059 & 0.0094 & 0.0019 & 0.0030\tabularnewline
\hline 
\multirow{4}{*}{2} & 0.90 & 0.8820 & 0.8895 & 0.8910 & 0.8960 & 0.8950 & 0.8950 & 0.9000 & 0.9000\tabularnewline
 & 0.95 & 0.9360 & 0.9425 & 0.9385 & 0.9390 & 0.9485 & 0.9495 & 0.9550 & 0.9550\tabularnewline
 & 0.975 & 0.9660 & 0.9685 & 0.9655 & 0.9665 & 0.9735 & 0.9735 & 0.9775 & 0.9780\tabularnewline
\cline{2-10} 
 & Avg. Ex. Len. & 0.0671 & 0.0678 & 0.0212 & 0.0213 & 0.0067 & 0.0068 & 0.0021 & 0.0021\tabularnewline
\hline 
\multirow{4}{*}{3} & 0.90 & 0.9190 & 0.9870 & 0.9225 & 0.9890 & 0.9140 & 0.9930 & 0.9160 & 0.9935\tabularnewline
 & 0.95 & 0.9550 & 0.9950 & 0.9595 & 0.9945 & 0.9560 & 0.9985 & 0.9515 & 0.9965\tabularnewline
 & 0.975 & 0.9760 & 0.9985 & 0.9800 & 0.9970 & 0.9785 & 0.9990 & 0.9685 & 0.9980\tabularnewline
\cline{2-10} 
 & Avg. Ex. Len. & 0.0630 & 0.0860 & 0.0195 & 0.0279 & 0.0061 & 0.0090 & 0.0019 & 0.0029\tabularnewline
\hline 
\multirow{4}{*}{4} & 0.90 & 0.8860 & 0.8860 & 0.8980 & 0.9005 & 0.8925 & 0.8925 & 0.8975 & 0.8975\tabularnewline
 & 0.95 & 0.9430 & 0.9430 & 0.9505 & 0.9515 & 0.9435 & 0.9470 & 0.9440 & 0.9440\tabularnewline
 & 0.975 & 0.9685 & 0.9685 & 0.9760 & 0.9780 & 0.9720 & 0.9730 & 0.9720 & 0.9720\tabularnewline
\cline{2-10} 
 & Avg. Ex. Len. & 0.0655 & 0.0721 & 0.0212 & 0.0220 & 0.0067 & 0.0068 & 0.0021 & 0.0021\tabularnewline
\hline 
\end{tabular}
\par\end{centering}
Note: Average excess length is measured as the difference between
the average $\left|\mbox{CI}_{\alpha,n}\right|$ and $\left|\setMarginal\right|$
for $\alpha=0.1$.
\end{table}
\par\end{center}
\newpage
